# Supplementary material for: Single pairs of time-bin entangled photons
Source: arXiv:1507.01876 source file (2015-07-07)
Supplement: Supplementary file 1 [file Versteegh_supplemental_material.pdf]

**Supplemental Material**

# Single pairs of time-bin entangled photons

Marijn A. M. Versteegh, Michael E. Reimer, Aafke A. van den Berg,
Gediminas Juska, Valeria Dimastrodonato, Agnieszka Gocalinska,
Emanuele Pelucchi, and Val Zwiller

## 1. Measurement of polarization entangled photon pairs

| | | | | | | | |
|---|---|---|---|---|---|---|---|
| HH | 642 | VH | 191 | DH | 384 | LH | 482 |
| HV | 188 | VV | 624 | DV | 277 | LV | 432 |
| HD | 460 | VD | 350 | DD | 716 | LD | 643 |
| HL | 409 | VL | 475 | DL | 481 | LL | 156 |

**Supplementary Table 1:** Polarization quantum state tomography. Measured numbers of coincidence counts within the selected time window of 3 ns for the indicated polarization selections, where the first letter indicates the XX polarization and the second letter indicates the X polarization. For this measurement the photons were sent directly to the tomography setup, without going through the interferometer. Calculation based on these results gives the following density matrix in the basis $\{|HH\rangle, |HV\rangle, |VH\rangle, |VV\rangle\}$:

$$\begin{pmatrix} 0.405 & 0.019 + 0.022i & -0.012 - 0.014i & 0.333 - 0.158i \\ 0.019 - 0.022i & 0.110 & 0.008 - 0.056i & -0.053 - 0.011i \\ -0.012 + 0.014i & 0.008 + 0.056i & 0.112 & -0.020 - 0.028i \\ 0.333 + 0.158i & -0.053 + 0.011i & -0.020 + 0.028i & 0.373 \end{pmatrix}.$$

This matrix is given in Figs. 5(b) and 5(c).

## 2. Measurement of time-bin entangled photon pairs

| | | | | | | | |
|---|---|---|---|---|---|---|---|
| HH | 34 | VH | 12 | DH | 30 | LH | 14 |
| HV | 12 | VV | 55 | DV | 26 | LV | 27 |
| HD | 30 | VD | 41 | DD | 30 | LD | 10 |
| HL | 31 | VL | 28 | DL | 15 | LL | 40 |

**Supplementary Table 2:** Time-bin quantum state tomography. Measured numbers of coincidence counts within the selected time window of 3 ns for the indicated polarization selections, where the first letter indicates the XX polarization and the second letter indicates

the X polarization. The photons were sent through the polarization-timebin interface to create the time-bin entanglement, and again through the interferometer for the time-bin tomography measurement. In this measurement *H* correponds to *l*, *V* corresponds to *e*, *D* correponds to $(l+e)/\sqrt{2}$ , and *L* corresponds to $(l-ie)/\sqrt{2}$ . Calculation based on these results gives the following density matrix in the basis $\{|ll\rangle, |le\rangle, |el\rangle, |ee\rangle\}$:

$$\begin{pmatrix} 0.303 & 0.071-0.067i & 0.054+0.069i & -0.178+0.297i \\ 0.071+0.067i & 0.106 & 0.060+0.057i & -0.063+0.037i \\ 0.054-0.069i & 0.060-0.057i & 0.108 & 0.071+0.048i \\ -0.178-0.297i & -0.063-0.037i & 0.071-0.048i & 0.483 \end{pmatrix}.$$

This matrix is given in Figs. 6(b) and 6(c).
